# Supplementary material for: Risk-Aware Scene Sampling for Dynamic Assurance of Autonomous Systems
Source: arXiv:2202.13510 source file (2022-02-28)
Supplement: Supplementary file 1 [file appendix.tex]

% \appendix
\newpage
\section*{Technical Appendix}

\subsection{Scene Specification File}
\cref{fig:file} shows the scene specification file that we use in the scene generation approach as discussed in \cref{sec:scene_generation}. As seen, this file provides a selection schema to select the scene variables and the sampler that they want to use for scene generation. This abstracts the user from directly interacting with the complexity of the language. In addition to the samplers discussed in the paper, we also have a manual sampling approach that will allow the user to manually type in values for the scene variables. 

\begin{figure}[!h]
 \centering
 \includegraphics[width=0.8\columnwidth]{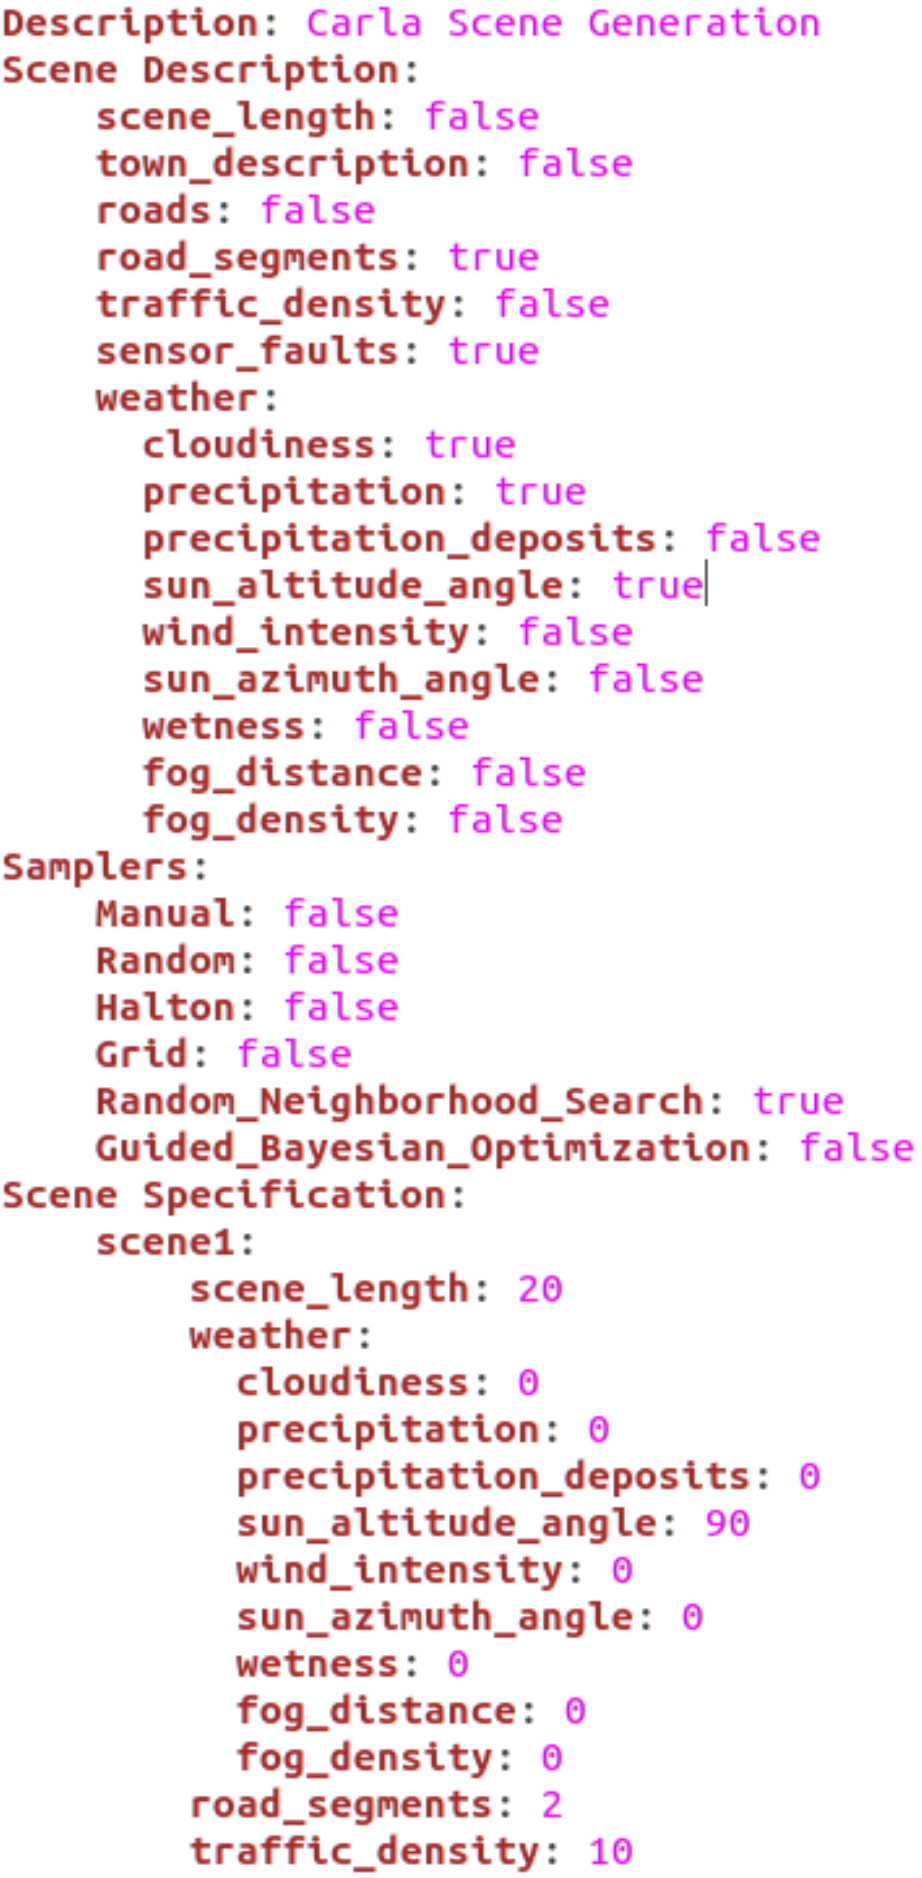}
 \caption{The specification file that we use with the scene generation approach.}
 \label{fig:file}
\end{figure}

\subsection{\ac{resonate} Risk Estimation}
Recall that we use the \ac{resonate} tool to estimate the system's dynamic risk or the \ac{resonate} score. For this, it estimates the hazard rate $\lambda$ and the likelihood of the hazard occurrence using a \ac{btd} as discussed in \cref{sec:risk_estimation}. \cref{fig:hazard_rate} illustrates the dynamic likelihood of a collision and the \ac{ood} detector results for two test scenes. Here, the risk estimator and the \ac{ood} detectors are used to estimate every simulation step. To explain, \textbf{Scene1} is a normal train scene with no adverse weather conditions. But it had two camera faults of left camera occlusion and right camera blur, which increased its likelihood of a collision. The average likelihood of a collision for the scene was $0.4$. Also, the \ac{av} did not perform any infractions in this scene. \textbf{Scene2} is a scene with high brightness. As seen, the likelihood of collision is high throughout the scene because the \ac{ood} detector identified the scene to be \ac{ood}. The average likelihood of a collision for the scene was $0.69$, and the system had an actual collision at $39^th$ second.

\begin{figure}[t]
 \centering
 \includegraphics[width=\columnwidth]{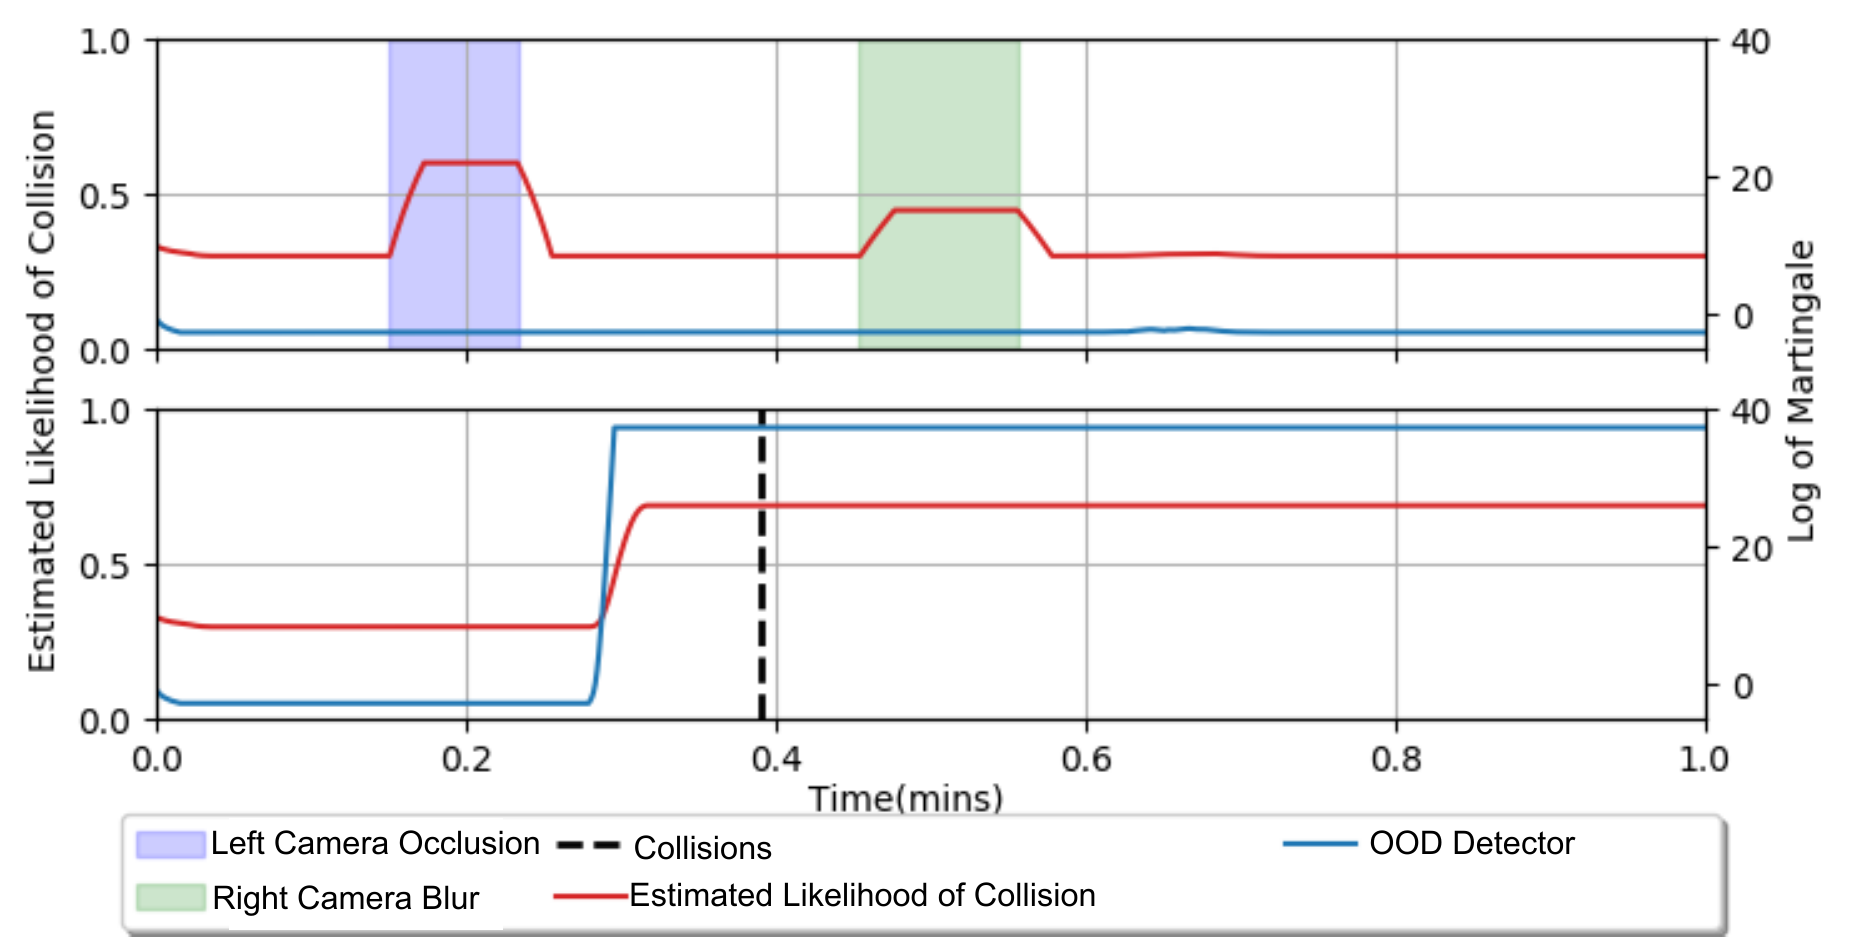}
 \caption{The estimated collision rate for two test scenes. (Top) Scene1 - A scene with two camera faults. The average likelihood of collision across the scene was $0.4$. (Bottom) Scene2 - A scene with adverse brightness. The average likelihood of collision across the scene was $0.69$.}
 \label{fig:hazard_rate}
%   \vspace{-0.15in}
\end{figure}

\subsection{Notation Lookup}

\begin{table}[!h]
    \centering

    \footnotesize
    \begin{tabular}{|c|p{7.2cm}|}
    \hline
    Notation & Description\\
    \hline
    $s$ & scene \\
    \hline
    $s_v$ & scene variables \\
    \hline
    $v_d$ & variable distribution \\
    \hline
    $v_c$ & variable constraints \\
    \hline
    $\mathbb{E}$ & Environmental variables \\
    \hline
    $\mathbb{S}$ & Structural variables \\
    \hline
    $\mathbb{F}$ & Fault variables \\
    \hline
    $\mathcal{SC}$ & Sampling Constraints \\
    \hline
    $\lambda$ & dynamic hazard rate \\
    \hline
    $S_{Risk}$ & Risk Score \\
    \hline
    $RS$ & \ac{resonate} Score \\
    \hline
    $IS$ & Infraction Score \\
    \hline
    $\delta$ & Risk threshold computed across calibration set \\
    \hline
    $\mathcal{E}$ & List of previously explored scenes \\
    \hline
    $k$ & \ac{rns} sampler's parameter to control exploration vs. exploitation \\
    \hline
    $\beta$ & \ac{gbo} sampler's parameter to control exploration vs. exploitation \\
    \hline
    $P$ & Precipitation \\
    \hline
    $C$ & Cloudiness \\
    \hline
    $T$ & Time-of-day \\
    \hline
    $RS$ & Road Segments \\
    \hline
    $TD$ & Traffic Density \\
    \hline
    \end{tabular}
    \caption{Symbols used in the paper}
    \label{Table:SymbolTable}
    % \vspace{-0.4em}
\end{table}
